# Supplementary material for: Distributed Deep Joint Source-Channel Coding with Decoder-Only Side Information
Source: arXiv:2310.04311 source file (2024-02-27)
Supplement: Supplementary file 1 [file appendix.tex]

\onecolumn

\appendix
